# Supplementary material for: Resolving Oversmoothing with Opinion Dissensus
Source: arXiv:2501.19089 source file (2025-05-16)
Supplement: Supplementary file 1 [file 4_additional_experiments.tex]

\begin{figure}[t]
    \centering
    \begin{minipage}{0.2\textwidth} % Left side (single figure)
        \centering
        \subfigure[Graph]{%
        \includegraphics[width=\textwidth]{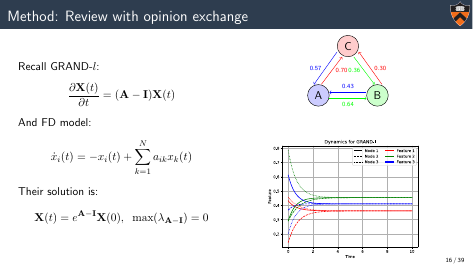} % Replace with your image
        }
    \end{minipage}
    \begin{minipage}{0.79\textwidth} % Right side (2x2 grid)
        \centering
        \begin{minipage}{0.45\textwidth}
            \centering
            \subfigure[GRAND-$\ell$]{%
                \includegraphics[width=\textwidth]{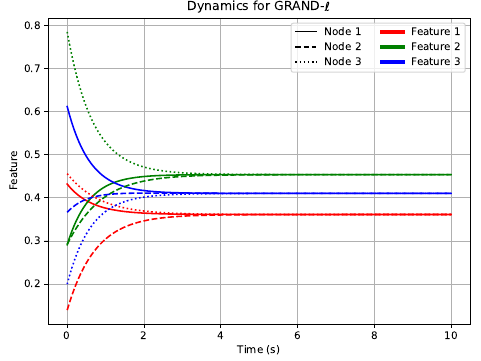} % Replace with your image
            }       
        \end{minipage}
        \begin{minipage}{0.45\textwidth}
            \centering
            \subfigure[GRAND++-$\ell$]{%
                \includegraphics[width=\textwidth]{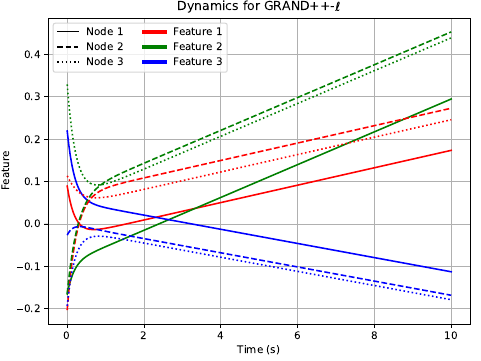} % Replace with your image
            }   
        \end{minipage}
        
        % \vspace{0.2cm} % Adjust spacing
        
        \begin{minipage}{0.45\textwidth}
            \centering
            \subfigure[GraphCON-Tran]{%
                \includegraphics[width=\textwidth]{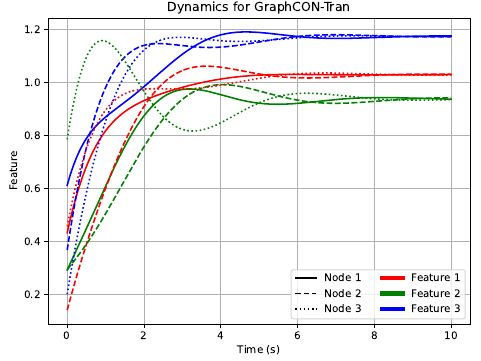} % Replace with your image
            }   
        \end{minipage}
        \begin{minipage}{0.45\textwidth}
            \centering
            \subfigure[BIMP (ours)]{%
                \includegraphics[width=\textwidth]{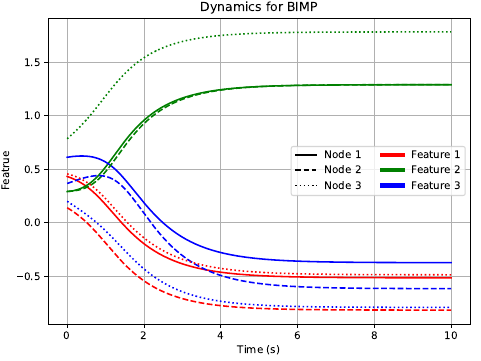} % Replace with your image
            }   
        \end{minipage}
    \end{minipage}
    
    \caption{\textbf{Toy simulations Result.} Given a fully connected graph shown in (a), we simulate and visualize the dynamics of GRAND-$\ell$, GRAND++-$\ell$, GraphCON-Tran and BIMP using the Euler method. All systems share the same adjacency matrix and initial state. The visualized result indicates all the methods, except BIMP, suffer from the oversmoothing as features for all three nodes converges to the same values.}
    \label{fig:simulation}
\end{figure}
\subsection{The Numerical Simulation Result}
In order to illustrate the shortcoming across the exiting methods while our method doesn't, we simulate a toy dynamics of: GRAND-$\ell$, GRAND++-$\ell$, GraphCON-Tran and BIMP. This visualization helps to understand the theoretical analysis in Section \ref{section:BINN}. The setting is   
% \begin{figure}[t]
%     \centering
%     % First Subfigure
%     \subfigure[GRAND-$\ell$]{%
%         \includegraphics[width=0.45\textwidth]{icml2024/figures/grand.pdf} % Replace with your image
%     }
%     % \hfill % Add horizontal space between subfigures
%     % Second Subfigure
%     \subfigure[GRAND++-$\ell$]{%
%         \includegraphics[width=0.45\textwidth]{icml2024/figures/grand++.pdf} % Replace with your image
%     }
%     % \hfill % Add horizontal space between subfigures
%     % Third Subfigure
%     \subfigure[GraphCON-Tran]{%
%         \includegraphics[width=0.45\textwidth]{icml2024/figures/GraphCON.pdf} % Replace with your image
%     }
%     % \hfill % Add horizontal space between subfigures
%     % Forth Subfigure
%     \subfigure[BIMP (ours)]{%
%         \includegraphics[width=0.45\textwidth]{icml2024/figures/nod.pdf} % Replace with your image
%     }
%     % Overall Caption
%     \caption{\color{blue}\textbf{Toy simulations Result.} Given a fully connected graph shown on the left, we simulate and visualize the dynamics (from upper left to lower right) of GRAND-$\ell$, GRAND++-$\ell$, GraphCON-Tran and BINN on this graph using the Euler method. All the dynamics systems share the same adjacency matrix and initial state. The visualized result indicates all the methods, except BIMP, suffer from the oversmoothing. }
%     \label{fig:simulation}
% \end{figure}
\begin{equation}
    \mathbf{A} =  \begin{bmatrix}
    0 & 0.43 & 0.57\\
    0.64 & 0 & 0.36\\
    0.70 & 0.30 & 0
    \end{bmatrix}, \quad
    \mathbf{X}(0) = \begin{bmatrix}
    0.43 & 0.29 & 0.61\\
    0.14 & 0.29 & 0.37\\
    0.46 & 0.79 & 0.20
    \end{bmatrix}.
\end{equation}
Particularly, in GRAND++-$\ell$, all the nodes are `trustworthy' to calculate the source term. In BIMP, we randomly generate the belief matrix $\mathbf{A}_\mathrm{o}$ using the same method as for $\mathbf{A}$.

In right side of Figure \ref{fig:simulation}, we present the simulated result for these four methods. We observe that features in GRAND-$\ell$ (upper left) quickly converge to the same values. In GraphCON-Tran (lower left), features also converge to the same but at slower speed rate due to its damping term resisting to the changes. Features in GRAND++-$\ell$ (upper right) remain a fixed difference between nodes after $t=4$, but this difference get ignorable over time, ultimately leading to feature similarity. In contract, BIMP keeps distinct features throughout and mitigates the oversmoothing.

% \begin{table}[h]
%     \centering
%     \caption{ \textbf{Classification accuracy on heterophilic datasets.} Classification accuracy on the Texas, Wisconsin and Cornell datasets. Our BIMP model outperforms most of the continuous-depth baselines.} 
%     \vskip 0.15in
%     \label{tab:heterophilic}
%     \begin{tabular}{cccc}
%         \toprule
%         Model &  Texas &  Wisconsin &  Cornell \\
%         \textit{Homophily level} & 0.11 & 0.21 & 0.30 \\
%         \midrule
%         BIMP (ours)  & \textbf{82.16$\pm$4.06} & \textbf{85.29$\pm$3.42} &  \textbf{77.13$\pm$3.38} \\
%         GRAND-$\ell$  & 74.59$\pm$5.43 & 82.75$\pm$3.90 & 70.00$\pm$6.22  \\
%         GraphCON-GCN & 80.54$\pm$4.49 & 84.79$\pm$2.51 & 74.05$\pm$3.24  \\
%         KuramotoGNN  &\underline{81.81$\pm$4.36} & \underline{85.09$\pm$4.42} & \underline{76.02$\pm$2.77} \\
%         % GCN & & &\\
%         % GAT & & &\\
%         \bottomrule
%     \end{tabular}
% \end{table}

\begin{table}[h]
    \centering
    \caption{ \textbf{Classification accuracy on heterophilic datasets.} Classification accuracy on the Texas, Wisconsin and Cornell datasets. Our BIMP model outperforms most of the continuous-depth baselines.} 
    \label{tab:heterophilic_full}
    \begin{tabular}{lccc}
        \hline
        Model &  Texas &  Wisconsin &  Cornell \\
        \textit{Homophily level} & 0.11 & 0.21 & 0.30 \\
        \hline
        \textbf{BIMP} & \textbf{82.16$\pm$4.06} & \textbf{85.29$\pm$3.42} & 77.13$\pm$3.38 \\
        \textbf{BIMP-aa} & 76.95$\pm$4.71 & 81.35$\pm$5.33 & \underline{\smash{85.30$\pm$4.90}} \\
        \textbf{BIMP-aa-rw} & 77.46$\pm$4.80 & 82.25$\pm$5.55 & \textbf{85.69$\pm$3.74} \\ \hdashline
        GRAND-$\ell$ & 74.59$\pm$5.43 & 82.75+3.90 & 70.00$\pm$6.22 \\
        GRAND-aa & 71.89$\pm$5.30 & 75.68$\pm$9.89 & 82.16$\pm$3.77 \\
        GRAND-aa-rw & 74.59$\pm$4.22 & 82.16$\pm$5.43 & 83.73$\pm$5.69 \\
        GRAND++-$\ell$ & 70.30$\pm$8.50 & 76.14$\pm$5.77 & 83.09$\pm$2.83 \\
        GRAND++-nl & 71.89$\pm$3.43 & 78.57$\pm$6.51 & 83.96$\pm$5.02 \\
        GRAND++-nl-rw & 74.05$\pm$5.57 & 79.42$\pm$5.24 & 84.62$\pm$3.56 \\
        KuramotoGNN & \underline{\smash{81.81$\pm$4.36}} & \underline{\smash{85.09$\pm$4.42}} & 76.02$\pm$2.77 \\
        GraphCON-GCN & 80.54$\pm$4.49 & 84.79$\pm$2.51 & 74.05$\pm$3.24 \\
        GAT & 42.16$\pm$7.07 & 57.84$\pm$5.82 & 49.61$\pm$4.21 \\
        GCN & 41.35$\pm$4.69 & 57.03$\pm$5.98 & 48.43$\pm$5.75 \\
        GCN-pairnorm & 52.70$\pm$6.42 & 63.51$\pm$6.54 & 60.59$\pm$4.34 \\
        GCN-group & 47.62$\pm$5.30 & 59.92$\pm$4.15 & 51.37$\pm$5.67 \\
        GraphSAGE & 70.54$\pm$2.55 & 72.70$\pm$5.47 & 73.14$\pm$6.27 \\
        \hline
    \end{tabular}
\end{table}

\subsection{Experiment on heterophilic datasets}\label{appendix:heterophilic}
We have evaluated our model on homophilic datasets in main paper, which holds the assumption that edges tend to connect similar nodes. However, many GNN models struggle with low accuracy on heterophilic datasets, where this assumption no longer holds. We deploy our BIMP model on three heterophilic datasets: \textbf{Texas, Wisconsin}, and \textbf{Cornell} from the CMU WebKB~\cite{craven1998learning} project. BIMP demonstrates competitive performance while maintaining low computational complexity.
%\footnote{https://www.cs.cmu.edu/afs/cs.cmu.edu/project/theo-11/www/wwkb/ \label{footnote}}

Table \ref{tab:heterophilic} lists the classification accuracy of BIMP and other continuous-depth GNNs on these heterophilic datasets. For all benchmarks, we run 10 fixed splits for each dataset with 20 random seeds for each split on work stations with an Intel Xeon Gold 5220R 24 core CPU, an Nvidia A6000 GPUs, and 256GB of RAM. The hyperparameters for BIMP are searched by Ray Tune process with 200 random trails. 

Our BIMP model outperforms baselines in all datasets, illustrating its improved performance on heterophilic datasets.

{\color{blue}
\subsection{Experiment on large graph}\label{appendix:large_graph}
To see how our model compares to baseline models on large graphs, we trained our BIMP model, GRAND-$\ell$, and KuramotoGNN on the ogbn-arXiv citation graph dataset \cite{hu2020open} across 10 ransom seeds, and got the classification accuracy reported in Table \ref{tab:large_graph}. These results suggest our approach performs on-par with continuous-depth GNNs on large graphs. 

The ogbn-axXiv dataset consists of a single graph with 169,343 nodes and 1,166,243 edges where each node represents an arxiv paper, and edges represent citation relationships. We train each model in a semi-supervised way, and compute the training loss over 90,941 of the 169,343 nodes. We use 29,799 of the remaining nodes for validation, and the final 48,603 nodes for testing.
\begin{table}[h]
    \centering
    \caption{ \textbf{Classification accuracy on ogbn-arXiv dataset.} Our BIMP model outperforms GRAND-$\ell$ and KuramotoGNN on the ogbn-arXiv dataset.} 
    \label{tab:large_graph}
    \begin{tabular}{lc}
        \hline
        Model & ogbn-arXiv  \\
        \hline
        \textbf{BIMP} &  \textbf{71.04$\pm$0.94} \\
        GRAND-$\ell$ & 70.19$\pm$0.43 \\
        KuramotoGNN & 66.96$\pm$0.25 \\
        \hline
    \end{tabular}
\end{table}

\subsection{Resilience to adversarial attack}
\label{experiment:attack}
%Assume there is a perturbation $\mathbf{\varepsilon}$ on initial embedding $\mathbf{X}(0)$. In GRAND-$\ell$ (Equation \eqref{eq:grand-l}), the perturbation would be applied on $\mathbf{A}$ directly. In contract, in BIMP, the saturating function $\text{tanh}(\cdot)$ smooths the effect of the perturbation.}

We demonstrate improved resilience to adversarial attack compared to GRAND-$\ell$ under random and PGD \cite{mkadry2017towards} attack methods on the Cora, Citeseer and Pubmed datasets. We use an untargeted graph modification attack, perturbingnode features at inference. In the random attack, we sample the perturbation from $\mathcal{N}(0,1)$, and in the PGD attack, we choose $\epsilon=0.03,\alpha = 0.01$. %For fairness, we set $d=1$ in BIMP making nonlinearity the only difference. 
Classification accuracies are reported in Table \ref{tab:performance_comparison}, and show that our BIMP model significantly outperforms the baseline model. {\color{blue} Should we add a brief explanation about BIMP's resilient to adversarial attacks?

Move to Appendix?}

\begin{table}[t]
    \centering
    \caption{\textbf{Robustness to adversarial attack.} Classification accuracy under different types of adversarial attacks are reported. BIMP shows significantly improved resilience to adversarial attacks compared to linear baseline models.}
    \begin{tabular}{lccc}
        \toprule
        Dataset & Attack method & BIMP (ours) & GRAND-$\ell$\\
        \midrule
        \multirow{3}{*}{Cora} 
        & Clean    & \textbf{82.4$\pm$2.1} & 82.1$\pm$1.4 \\
        & Random  & \textbf{70.8$\pm$1.6} & 61.6$\pm$2.3 \\
        & PGD   & \textbf{56.4$\pm$5.4} & 38.4$\pm$4.9  \\
        \midrule
        \multirow{3}{*}{Citeseer} 
        & Clean    & \textbf{70.4$\pm$1.6} & 70.0$\pm$1.7 \\
        & Random   & \textbf{57.8$\pm$1.2} & 42.5$\pm$2.2 \\
        & PGD   & \textbf{57.4$\pm$3.1} & 39.6$\pm$3.7 \\
        \midrule
        \multirow{3}{*}{Pubmed} 
        & Clean   & \textbf{79.7$\pm$1.9} & 78.3$\pm$2.1 \\
        & Random  & \textbf{61.2$\pm$6.7} & 40.8$\pm$2.5 \\
        & PGD     & \textbf{40.1$\pm$7.8} & 37.6$\pm$5.6 \\
        \bottomrule
    \end{tabular}
    \label{tab:performance_comparison}
    \vskip -0.15in
\end{table}

}
{\color{blue}
\subsection{Choice of nonlinearity in NOD module}\label{appendix:nonlinearity}
To understand how the choice of nonlinearity in our Nonlinear Opinion Dynamics (NOD) module impacts performance, we experiment with a suite of alternative nonlinearities (softsign, arctan, sigmoid, ReLu, Leaky ReLu, and GeLu) and linearity (linear). Softsign and arctan satisfy the nonlinearity constraint in the NOD definition (i.e., $S(0)=0, S'(0)=1, S''(0)\neq0$), but sigmoid, ReLu, Leaky ReLu, and GeLu do not. Specifically, sigmoid does not pass through the origin, ReLu and Leaky ReLu are not differentiable, and GeLu does not satisfy $S'(0)=1$. Linear refers to the BIMP model without any nonlinearity. We find that using nonlinearities that meet the NOD criteria effectively prevent oversmoothing, while the others do not. We report the classification accuracy of our BIMP model with alternative nonlinearities in the NOD module in Table \ref{table:nonlinearity}.
}
\begin{table}[h]
    \centering
    \caption{\textbf{NOD nonlinearity}.Classification accuracy of our BIMP model on the Cora dataset using softsign, arctan, sigmoid, ReLu, Leaky ReLu, GeLu and linear is reported.}
    \vspace{3mm}
    \setlength\tabcolsep{3pt}
    \label{table:nonlinearity}
    \begin{tabular}{lcccccccc}
    \hline
    Layer & 1 & 2 & 4 & 8 & 16 & 32 & 64 & 128\\
    \hline
    tanh 
     & \underline{\smash{69.96$\pm$1.45}} & \underline{\smash{75.00$\pm$1.50}} & \underline{\smash{79.93$\pm$1.41}} & \textbf{82.21$\pm$1.26} & \textbf{82.83$\pm$1.12} & \textbf{82.81$\pm$1.19} & \underline{82.53$\pm$1.07} & \textbf{82.18$\pm$1.06}\\
    softsign
     & 63.25$\pm$1.73 & 68.34$\pm$2.03 & 72.37$\pm$1.50 & 77.05$\pm$1.67 & 79.88$\pm$1.82 & 81.45$\pm$1.48 & 81.14$\pm$1.65 & \underline{81.71$\pm$1.37}\\
    arctan
     & 64.05$\pm$1.58 & 72.62$\pm$2.40 & 76.91$\pm$1.82 & 79.84$\pm$1.05 & 81.81$\pm$1.54 & 82.48$\pm$1.81 & \textbf{82.94$\pm$0.73} & 81.26$\pm$1.93\\ \hdashline
    sigmoid
     & 60.36$\pm$1.39 & 63.20$\pm$1.63 & 65.54$\pm$1.80 & 63.91$\pm$2.13 & 29.55$\pm$1.80 & 29.92$\pm$1.22 & 30.72$\pm$1.02 & 29.37$\pm$2.77\\
    ReLu
     & 64.17$\pm$1.72 & 67.21$\pm$2.18 & 73.16$\pm$1.44 & 77.76$\pm$1.47 & 81.32$\pm$0.96 & 82.51$\pm$1.51 & 76.56$\pm$3.88 & 71.18$\pm$7.09\\
    LeakyReLu
     & 65.21$\pm$1.96 & 69.10$\pm$1.54 & 75.04$\pm$0.79 & 79.59$\pm$2.10 & \underline{\smash{82.04$\pm$1.50}} & \underline{\smash{82.58$\pm$1.17}} & 78.96$\pm$2.51 & 71.10$\pm$5.96\\
    GELU
     & 62.45$\pm$1.57 & 67.06$\pm$2.25 & 72.40$\pm$1.60 & 77.56$\pm$1.49 & 81.47$\pm$0.63 & 27.99$\pm$4.22 & 29.64$\pm$1.82 & 26.27$\pm$4.89\\
    linear
     & \textbf{77.52$\pm$1.44} & \textbf{81.92$\pm$0.85} & \textbf{82.08$\pm$1.34} & \underline{\smash{81.24$\pm$1.48}} & 80.45$\pm$1.43 & 79.99$\pm$1.21 & 76.74$\pm$1.86 & 75.44$\pm$0.89\\
    \hline
    \end{tabular}
    \vspace{-0.1in}
\end{table}
